# Supplementary material for: Temp-SCONE: A Novel Out-of-Distribution Detection and Domain Generalization Framework for Wild Data with Temporal Shift
Source: arXiv:2512.04571 source file (2025-12-04)
Supplement: Supplementary file 1 [file Appendix.tex]

\usepackage{graphicx}
\usepackage{caption}
\usepackage{subcaption} % if you want subfigures

\section{Additional Results}

\begin{figure}[htbp]
    \centering
    \includegraphics[width=0.8\textwidth]{Distinct_Dataset_experiments/Job1/Job_1_Covaria...png}
    \caption{Covariate shift results for Job 1}
    \label{fig:job1-covariate}
\end{figure}

\begin{figure}[htbp]
    \centering
    \includegraphics[width=0.8\textwidth]{Distinct_Dataset_experiments/Job2/Job_2_Covaria...png}
    \caption{Covariate shift results for Job 2}
    \label{fig:job2-covariate}
\end{figure}

\begin{figure}[htbp]
    \centering
    \includegraphics[width=0.8\textwidth]{Distinct_Dataset_experiments/Job3/Job_3_Covaria...png}
    \caption{Covariate shift results for Job 3}
    \label{fig:job3-covariate}
\end{figure}
